# Supplementary material for: Deterring Searches for Child Sexual Abuse Material on Google Search and Promoting Help-Seeking
Source: arXiv:2606.06126 source file (2026-06-05)
Supplement: Supplementary file 1 [file Supplemental.tex]

\documentclass[11pt]{article}

% --- Essential Packages ---
\usepackage[utf8]{inputenc}
\usepackage[T1]{fontenc}
\usepackage{geometry}
\geometry{a4paper, margin=1in}
\usepackage{booktabs} % Required for \toprule, \midrule, \bottomrule
\usepackage{caption}  % For better table captions
\usepackage{float}    % To force table placement with [H]
\usepackage{xurl}
\usepackage{booktabs}
\usepackage{threeparttable}
\usepackage{subcaption}
\usepackage{enumitem}
\usepackage{tabularx}
% --- Document Metadata ---
\title{Supplemental Material}
\date{} % Suppresses the date
\begin{document}

\maketitle

\appendix
%\section{Supplemental Material}

% Ensure the relative paths 'Tables/STOP.tex' and 'Tables/vpn.tex' 
% exist in your local directory.

\input{Tables/STOP}

\newpage

\input{Tables/vpn}

\end{document}
